# Supplementary material for: LanSER: Language-Model Supported Speech Emotion Recognition
Source: arXiv:2309.03978 source file (2023-09-07)
Supplement: Supplementary file 1 [file appendix.tex]

\section{Appendix}

- Preliminary experiments for incorporating contexts

- Extracted weak-label distributions for large-scale datasets

-Full taxonomy
